# Supplementary material for: An End-to-End Framework for Optimizing Foot Trajectory and Force in Dry Adhesion Legged Wall-Climbing Robots
Source: arXiv:2504.19448 source file (2025-05-08)
Supplement: Supplementary file 1 [file 0X_appendix.tex]

\appendix
\section{Appendix}
\label{app:localdiff}

We present here the formulation of the diffusion process as a \emph{local} denoising, as discussed and used in prior work~\cite{lidiff,scorelidar}. 
We then highlight our concerns, arguing that this approach can be more complex and may introduce approximations in the denoising process.

\subsection{Formulation of the diffusion process as a local denoising}

{Starting from a dense point cloud $\mathbf{p}_0^d$, the forward process in LiDiff~\cite{lidiff} satisfies

\begin{align}
\label{eq:forward_lidiff}
\mathbf{p}_t^d = \mathbf{p}_0^d + \sqrt{1 - \bar{\alpha}_t} \; \mathbf{\epsilon},
\end{align}
which is obtained by {considering point offsets with respect to the ground truth $\mathbf{p}_0^d$,} setting 
\begin{align}
\label{eq:link_x_p}
\mathbf{x}_t = \mathbf{p}_t^d  - \mathbf{p}_0^d \quad \text{and}  \quad \mathbf{x}_0 = \mathbf{0} 
\end{align}
in \cref{eq:forward}. The endpoint of this forward local diffusion process, or, equivalently, the starting point of the reverse denoising process, $\mathbf{p}_T^d$, is thus a noisy version of $\mathbf{p}_0^d$.

Second, conditioning $\epsilon_\theta$ on $\mathbf{x}_t$ as in 
\cref{eq:learned_neural_net} is not possible as it would require knowing $\mathbf{p}_0^d$ during generation. Therefore, $\epsilon_\theta$ is instead conditioned on $\mathbf{p}_t^d$ and trained to minimize
\begin{align}
\label{eq:learned_neural_net_lidff}
& \mathcal{L}(\theta) 
= 
\mathbb{E}_{\mathbf{p}^d_t} \left[ \| \mathbf{\epsilon} - \epsilon_\theta(\mathbf{p}^d_t, t) \|^2 
+ \lambda \, \mathcal{L}_{\rm reg}(\epsilon_\theta(\mathbf{p}^d_t, t))\right],\\
& \text{with}\;
 \mathcal{L}_{\rm reg}(\epsilon_\theta(\mathbf{p}^d_t, t)) 
= \mathcal{L}_{\rm mean}(\epsilon_\theta(\mathbf{p}^d_t, t))
+ \mathcal{L}_{\rm std}(\epsilon_\theta(\mathbf{p}^d_t, t))\,,\nonumber
\end{align}
where $\lambda>0$, and $\mathcal{L}_{\rm mean},\mathcal{L}_{\rm std}$ return the mean and standard deviation of the entries in $\epsilon_\theta(\mathbf{p}^d_t, t)$. 
When setting $\lambda=0$, the LiDiff authors noticed that the mean and standard deviation of $\epsilon_\theta$ were far from $0$ and $1$, while $\mathbf{\epsilon} \sim \mathcal{N}(\mathbf{0}, \mathbf{I})$. 
Thus, the regularization loss $\mathcal{L}_{\rm reg}$ was introduced to guide the outputs of $\epsilon_\theta$ towards these expected values.
 
Third, using Eqs. (\ref{eq:link_x_p}) in (\ref{eq:denoising}), the reverse denoising becomes
\begin{align}
\label{eq:pdt}
\mathbf{p}_{t-1}^d 
= 
\mathbf{p}_{0}^d 
+ 
\frac{\mathbf{p}_{t}^d - \mathbf{p}_{0}^d}{\sqrt{\alpha_t}} 
- 
\frac{(1 - \alpha_t) \, \epsilon_\theta(\mathbf{p}^d_t, t)}{\sqrt{\alpha_t \, (1 - \bar{\alpha}_t)}}  
+ 
\sqrt{\beta_t} \; \mathbf{z}\,.
\end{align}
Yet, this formula is unusable in practice as it requires access to the dense ground-truth point cloud $\mathbf{p}_{0}^d$, which is unknown during generation. As a workaround, LiDiff replaces
the dense point cloud $\mathbf{p}_{0}^d$ by a noisy estimate $\tilde{\mathbf{p}}^s$, %
obtained by noising $K$ duplications of the sparse point cloud $\mathbf{p}^s$. 
Ultimately, the approximate reverse denoising process writes
\begin{align}
\label{eq:denoising_lidiff}
\mathbf{p}_{t-1}^d 
= 
\tilde{\mathbf{p}}^s
+ 
\frac{\mathbf{p}_{t}^d - \tilde{\mathbf{p}}^s}{\sqrt{\alpha_t}} 
- 
\frac{(1 - \alpha_t) \, \epsilon_\theta(\mathbf{p}^d_t, t)}{\sqrt{\alpha_t \, (1 - \bar{\alpha}_t)}}  
+ 
\sqrt{\beta_t} \; \mathbf{z}\,.
\end{align}

Finally, one needs to construct a starting point $\mathbf{p}_T^d$ of the reverse denoising process. 
According to the forward process in \cref{eq:forward_lidiff}, a starting point can be constructed by sampling $\mathbf{z} \sim \mathcal{N}(\mathbf{0}, \mathbf{I})$ and adding it to $\mathbf{p}_0^d$, \ie, 
\begin{align}
\mathbf{p}_T^d 
= \mathbf{p}_0^d + \sqrt{1 - \bar{\alpha}_T} \; \mathbf{z}
\,\simeq\, \mathbf{p}_0^d + \mathbf{z},
\end{align}
where we use the fact that $\sqrt{1 - \bar{\alpha}_T} \simeq 1$, as in vanilla DDPM. Again, it would require knowing the ground truth $\mathbf{p}_0^d$. Instead, the starting point is also approximated  using $\tilde{\mathbf{p}}^s$:
\begin{align}
\label{eq:start_lidiff}
\mathbf{p}_T^d = \tilde{\mathbf{p}}^s 
+ \mathbf{z}, \quad \text{ where } \quad \mathbf{z} \sim \mathcal{N}(\mathbf{0}, \mathbf{I}).
\end{align}
}

\subsection{Limitations of local denoising paradigm}

While the above local point diffusion proved to work, it holds on major approximations, which we outline here.

\textbf{a.~}The justification of LiDiff to propose local point diffusion is that DDPM requires normalization, which leads to compression of data along some of the point cloud axes (Sec.~3.3 of LiDiff~\cite{lidiff}). 
We believe this observation may be flawed.
Not only could normalization be applied within fixed bounds, but it is actually not needed for DDPM, which can be formulated in the metric space (see~\cref{sec:meth_meth}).

\textbf{b.~}A major limitation of local diffusion is the reliance on a noisy estimate $\tilde{\mathbf{p}}^s$ of the ground truth in \cref{eq:pdt} and \cref{eq:start_lidiff}, which hinders its use for data generation, thereby losing one of the major properties of diffusion models.

\textbf{c.~}Third, diffusion requires the predicted noise to converge to a zero-centered distribution. To compensate for the predicted local noise not being zero-centered, the authors add an additional regularization term $\mathcal{L}_{\rm reg}$ (Sec.~3.4 of LiDiff~\cite{lidiff}), which further complexifies the optimization objective.

In this work, we show that DDPM can be applied on non-normalized point clouds without losing details after generation. Hence, the local (re-)formulation is not required (observation \textbf{a.}).
Moreover, since we follow the vanilla `scene-level' diffusion, our formulation does not require any additional regularization (observation \textbf{b.}). Last, a byproduct of our choices is that our simpler formulation opens up the possibility to generate point clouds %
(observation \textbf{c.}).

\section*{Acknowledgment}

This work has been carried out using HPC resources from GENCI-IDRIS (grants AD011014484R1, AD011012883R3).
We thank Mickael Chen, Corentin Sautier and Mohammad Fahes for the proofreading and valuable feedback.
